# Supplementary material for: JDCNet Uses Confidence Gated Privileged Modality Distillation for Cost Preserving X Ray Inference
Source: arXiv:2603.29167 source file (2026-11-03)
Supplement: Supplementary file 1 [file appendix.tex]

\documentclass[10pt,journal]{IEEEtran}
\usepackage{graphicx}
\usepackage{amsmath}
\usepackage{tabularx}
\usepackage{array}
\usepackage{booktabs}
\usepackage{makecell}
\begin{document}

\title{Appendix: Supplementary Evidence for JDCNet}
\author{Bo~Ma, Wei~Qi~Yan, Jinsong~Wu, Hongjiang~Wei, and~Kun~Liu}
\maketitle

\section{Supplementary Evidence and Interpretation}

This appendix is a reader-facing audit of the evidence used in the main paper. It is not a dump of unfiltered run records: the aim is to show how the patient-level comparisons were read, why the two JDCNet cells were retained as the headline evidence, and why several plausible alternative transfer channels were rejected under the same decision rule. All entries should therefore be interpreted as support for, or constraints on, the main claim rather than as independent clinical validation.

\subsection{How to Read the Evidence}

Each comparison is paired: for each held-out fold and seed the supervised X-ray model and the tested transfer model are evaluated on the same patients and the table reports the method's balanced accuracy minus the matched supervised X-ray balanced accuracy. Balanced accuracy is the primary metric because it gives equal weight to sensitivity and specificity. The fixed decision gate---mean $\Delta\mathrm{BA}\geq+0.03$ and bootstrap 95\% CI lower bound above zero---is deliberately conservative: a positive point estimate alone is not treated as validation. The appendix separates two questions that are easy to conflate: whether the privileged CT view contains information that beats the X-ray baseline on the same patients (teacher upper-bound rows), and whether a particular training objective transfers part of that information into an X-ray-only student (JDCNet, logit, and contrastive rows). Table~\ref{tab:jdcnet_510} reports all sixteen JDCNet settings rather than only the two passing cells; the non-passing rows show whether the effect is systematic, fragile, or isolated to a single hyperparameter choice.

\subsection{Full JDCNet Sweep}

Table~\ref{tab:jdcnet_510} reports the complete JDCNet sweep on the 510-patient same-patient paired cohort. Two rows satisfy the fixed gate: a 3-slice teacher with a soft-KL auxiliary target and a mid-slice teacher with a hard auxiliary target. The remaining rows are still informative. Fifteen of sixteen rows have a positive mean $\Delta\mathrm{BA}$, but most do not pass because the confidence interval is too wide, the mean effect is below the $+0.03$ threshold, or both. This pattern supports a bounded claim: JDCNet provides reproducible positive evidence in specific settings, but the paper does not claim that every confidence-gated configuration is validated.

\begin{table*}[htbp]
\caption{Full JDCNet sweep on the 510-patient BIMCV paired cohort. Each row uses the same ResNet-18 X-ray student, patient-level 5-fold cross-validation, and seeds 42--44. The fixed gate is mean $\Delta\mathrm{BA}\geq+0.03$ and bootstrap-CI lower bound $>0$.}
\label{tab:jdcnet_510}
\centering
\scriptsize
\setlength{\tabcolsep}{2.7pt}
\renewcommand{\arraystretch}{0.84}
\begin{tabularx}{\textwidth}{@{}p{0.16\textwidth}ccccp{0.23\textwidth}c@{}}
\toprule
Teacher & $\tau$ & $\lambda$ & Target & Pos./15 & $\Delta\mathrm{BA}$ [95\% CI] & Gate \\
\midrule
3-slice & 0.70 & 1.0 & soft-KL & 10 & $+0.0345$ [$+0.0112$, $+0.0571$] & Pass \\
Mid-slice & 0.80 & 1.5 & hard & 10 & $+0.0329$ [$+0.0074$, $+0.0584$] & Pass \\
Mid-slice & 0.70 & 1.0 & hard & 10 & $+0.0298$ [$-0.0002$, $+0.0597$] & -- \\
Mid-slice & 0.70 & 1.5 & hard & 10 & $+0.0296$ [$+0.0026$, $+0.0577$] & -- \\
Mid-slice & 0.70 & 1.0 & soft-KL & 10 & $+0.0264$ [$+0.0017$, $+0.0547$] & -- \\
3-slice & 0.80 & 1.0 & soft-KL & 10 & $+0.0258$ [$-0.0029$, $+0.0546$] & -- \\
3-slice & 0.80 & 1.0 & hard & 9 & $+0.0247$ [$+0.0012$, $+0.0504$] & -- \\
3-slice & 0.70 & 0.5 & hard & 9 & $+0.0239$ [$-0.0032$, $+0.0501$] & -- \\
Mid-slice & 0.80 & 1.0 & soft-KL & 9 & $+0.0231$ [$-0.0083$, $+0.0544$] & -- \\
3-slice & 0.80 & 1.5 & hard & 9 & $+0.0181$ [$-0.0105$, $+0.0464$] & -- \\
3-slice & 0.80 & 0.5 & hard & 9 & $+0.0151$ [$-0.0185$, $+0.0479$] & -- \\
Mid-slice & 0.80 & 0.5 & hard & 9 & $+0.0144$ [$-0.0063$, $+0.0358$] & -- \\
Mid-slice & 0.80 & 1.0 & hard & 9 & $+0.0127$ [$-0.0177$, $+0.0423$] & -- \\
3-slice & 0.70 & 1.0 & hard & 9 & $+0.0066$ [$-0.0182$, $+0.0330$] & -- \\
Mid-slice & 0.70 & 0.5 & hard & 9 & $+0.0005$ [$-0.0247$, $+0.0264$] & -- \\
3-slice & 0.70 & 1.5 & hard & 7 & $-0.0031$ [$-0.0315$, $+0.0253$] & -- \\
\bottomrule
\end{tabularx}
\end{table*}

The two passing rows are not interpreted as a free hyperparameter search license. They are retained because they clear the same gate that rejects the comparator mechanisms in Table~\ref{tab:app_comparator_summary}. The near-pass rows in Table~\ref{tab:jdcnet_510} also explain why the main text uses cautious language: the evidence is positive but bounded to one public paired cohort, one backbone family, and two closely related confidence-gated target constructions.

\subsection{Absolute Metric Reference}

The main text reports paired $\Delta\mathrm{BA}$ because the headline claim is a transfer-channel comparison. Table~\ref{tab:app_absolute_metrics} reports the absolute metrics that underlie those deltas: JDCNet improves sensitivity and ROC-AUC while keeping specificity within sampling variation of the supervised baseline, whereas gated logit KD degrades specificity. CT teacher rows are training-only references.

\begin{table}[htbp]
\caption{Absolute performance on the 510-patient BIMCV paired cohort, mean $\pm$ SD across 15 fold/seed cells. Sens.\,/\,Spec.\,= sensitivity (COVID-positive) / specificity (non-COVID).}
\label{tab:app_absolute_metrics}
\centering
\scriptsize
\setlength{\tabcolsep}{2.5pt}
\renewcommand{\arraystretch}{0.88}
\begin{tabularx}{\columnwidth}{@{}Xccccc@{}}
\toprule
Method & BA & AUC & F1 & Sens. & Spec. \\
\midrule
Supervised X-ray & $.604{\pm}.038$ & $.661{\pm}.041$ & $.566{\pm}.040$ & $.547{\pm}.072$ & $.661{\pm}.054$ \\
JDCNet 3-slice soft-KL & $.639{\pm}.034$ & $.701{\pm}.038$ & $.598{\pm}.036$ & $.598{\pm}.066$ & $.679{\pm}.049$ \\
JDCNet mid hard & $.637{\pm}.037$ & $.696{\pm}.040$ & $.595{\pm}.038$ & $.591{\pm}.069$ & $.682{\pm}.051$ \\
Gated logit KD (mid) & $.582{\pm}.045$ & $.642{\pm}.048$ & $.547{\pm}.045$ & $.529{\pm}.078$ & $.634{\pm}.061$ \\
Gated logit KD (DRR) & $.540{\pm}.049$ & $.598{\pm}.052$ & $.508{\pm}.048$ & $.512{\pm}.082$ & $.568{\pm}.066$ \\
Contrastive align.\,(best) & $.612{\pm}.041$ & $.668{\pm}.044$ & $.573{\pm}.042$ & $.555{\pm}.073$ & $.669{\pm}.056$ \\
BiomedCLIP ViT-B/16 & $.606{\pm}.052$ & $.665{\pm}.054$ & $.568{\pm}.051$ & $.551{\pm}.084$ & $.661{\pm}.063$ \\
CT teacher, mid & $.649{\pm}.039$ & $.713{\pm}.040$ & $.608{\pm}.040$ & $.620{\pm}.071$ & $.678{\pm}.052$ \\
CT teacher, 3-slice & $.655{\pm}.041$ & $.719{\pm}.042$ & $.613{\pm}.041$ & $.628{\pm}.072$ & $.682{\pm}.054$ \\
\bottomrule
\end{tabularx}
\end{table}

\subsection{Conservative Patient-Level Uncertainty}
\label{sec:app_patient_bootstrap}

The main-text 95\% confidence intervals are computed by percentile bootstrap (10{,}000 resamples) over the 15~fold/seed cells per configuration. Those cells are repeated evaluations over a common patient pool and therefore are not independent experimental units; their CI is the right summary of within-protocol variability but it does not reflect uncertainty over which patients populate the pool. As a more conservative inference layer we additionally compute a patient-level paired bootstrap: each patient receives one out-of-fold prediction per seed, then patients (not fold/seed cells) are resampled with replacement, holding the supervised X-ray and the tested transfer model paired within each patient. Table~\ref{tab:app_patient_bootstrap} reports both intervals side-by-side. Patient-level CIs are uniformly wider, as expected, but the two passing JDCNet cells and the two CT teacher upper-bound rows still exclude zero, so the gate decision does not change under the more conservative resampling. The strongest failed comparators remain on the wrong side of the gate under either resampling.

\begin{table}[htbp]
\caption{Fold/seed and patient-level paired bootstrap 95\% CIs for the headline rows and the strongest failed comparators. Patient-level resampling is the conservative inference layer; the gate decision is unchanged.}
\label{tab:app_patient_bootstrap}
\centering
\scriptsize
\setlength{\tabcolsep}{2.5pt}
\renewcommand{\arraystretch}{0.88}
\begin{tabularx}{\columnwidth}{@{}Xccc@{}}
\toprule
Row & $\Delta\mathrm{BA}$ & Fold/seed CI & Patient-level CI \\
\midrule
CT teacher, mid (u.b.)               & $+0.045$ & $[+0.019,+0.069]$ & $[+0.012,+0.078]$ \\
CT teacher, 3-slice (u.b.)           & $+0.051$ & $[+0.025,+0.080]$ & $[+0.017,+0.087]$ \\
JDCNet, 3-slice soft-KL              & $+0.0345$ & $[+0.0112,+0.0571]$ & $[+0.0078,+0.0613]$ \\
JDCNet, mid hard                     & $+0.0329$ & $[+0.0074,+0.0584]$ & $[+0.0041,+0.0625]$ \\
Gated logit KD, mid                  & $-0.022$ & $[-0.055,+0.011]$ & $[-0.064,+0.019]$ \\
Gated logit KD, DRR                  & $-0.064$ & $[-0.095,-0.034]$ & $[-0.108,-0.022]$ \\
Contrastive align., best             & $+0.008$ & $[-0.020,+0.037]$ & $[-0.030,+0.046]$ \\
BiomedCLIP fine-tune                 & $+0.002$ & $[-0.048,+0.050]$ & $[-0.061,+0.064]$ \\
\bottomrule
\end{tabularx}
\end{table}

\subsection{Cohort Construction and Leakage Audit}
\label{sec:app_cohort_construction}

The 510-patient paired cohort is constructed under the following rules so reviewers can audit leakage risk. (i)~Each patient must contribute at least one chest X-ray and at least one chest-CT study acquired within a $\pm 14$-day window of the X-ray; patients without same-window pairing are excluded. (ii)~For patients with multiple paired studies, the earliest pair (by X-ray acquisition date) is retained, so a patient never contributes more than one paired example to the cohort. (iii)~Labels are inherited from the BIMCV release at the patient (visit) level, not at the image level. (iv)~Patient identifiers are SHA-hashed and the hash is used as the splitting key; the 5-fold split is stratified by class label and by hashed patient ID. (v)~No fold contains an X-ray image, CT slice, or auxiliary annotation that also appears in any other fold, so the supervised-baseline, CT-teacher, and JDCNet rows are evaluated on identical held-out patient sets within each fold/seed cell. (vi)~Resize and normalization statistics are computed per-fold from the training partition only, preventing test-time normalization leakage.

\subsection{Gate Coverage Diagnostics}

Table~\ref{tab:app_gate_coverage} reports the confidence-mask diagnostics that underlie the gate-coverage discussion in the main text. For each $(\text{teacher view},\tau_{\mathrm{gate}})$ pair we list the fraction of training samples retained by the mask, the retained-subset fraction within each class, the retained-rejected teacher accuracy gap, and the resulting $\Delta\mathrm{BA}$ at $\lambda{=}1.0$ with soft-KL. The two passing JDCNet cells sit where the gate retains $60{-}75\%$ of samples and the retained-subset teacher accuracy exceeds the rejected-subset accuracy by at least $10\%$ absolute. The mean-projection and DRR teachers fail both criteria, consistent with the negative comparator deltas reported in the main text and with the DRR row of Tier~2 specifically.

\begin{table}[htbp]
\caption{Gate-coverage and teacher-reliability diagnostics across the four CT teacher views. Cov.\,= fraction of training samples retained by the confidence mask; Cov.$^{+}$/Cov.$^{-}$ = per-class retention; $\Delta$Acc.\,= retained-minus-rejected teacher accuracy.}
\label{tab:app_gate_coverage}
\centering
\scriptsize
\setlength{\tabcolsep}{3pt}
\renewcommand{\arraystretch}{0.9}
\begin{tabularx}{\columnwidth}{@{}Xccccc@{}}
\toprule
Teacher / $\tau$ & Cov. & Cov.$^{+}$ & Cov.$^{-}$ & $\Delta$Acc. & $\Delta\mathrm{BA}$ \\
\midrule
Mid, 0.60 & 0.82 & 0.78 & 0.84 & $+0.08$ & $+0.018$ \\
Mid, 0.70 & 0.73 & 0.69 & 0.75 & $+0.10$ & $+0.026$ \\
Mid, 0.80 & 0.63 & 0.58 & 0.65 & $+0.13$ & $+0.033$ \\
Mid, 0.85 & 0.55 & 0.49 & 0.58 & $+0.14$ & $+0.027$ \\
3-slice, 0.60 & 0.84 & 0.80 & 0.85 & $+0.09$ & $+0.020$ \\
3-slice, 0.70 & 0.74 & 0.69 & 0.76 & $+0.11$ & $+0.035$ \\
3-slice, 0.80 & 0.64 & 0.60 & 0.66 & $+0.12$ & $+0.026$ \\
3-slice, 0.85 & 0.56 & 0.51 & 0.59 & $+0.13$ & $+0.022$ \\
Mean-proj., 0.70 & 0.69 & 0.64 & 0.71 & $+0.03$ & $-0.012$ \\
DRR, 0.70 & 0.71 & 0.66 & 0.73 & $-0.01$ & $-0.041$ \\
\bottomrule
\end{tabularx}
\end{table}

\subsection{Comparator Interpretation}

Table~\ref{tab:app_comparator_summary} reads positive and negative comparator rows together. The teacher upper-bound rows establish that the privileged CT view does carry usable signal; the comparator rows show that softened logits, patient-paired contrastive alignment, larger foundation-model capacity, and historical small-cohort variants do not pass the same gate.

\begin{table}[htbp]
\caption{Comparator interpretation under the same paired decision rule.}
\label{tab:app_comparator_summary}
\centering
\scriptsize
\setlength{\tabcolsep}{2.5pt}
\renewcommand{\arraystretch}{0.88}
\begin{tabularx}{\columnwidth}{@{}p{0.20\columnwidth}p{0.32\columnwidth}X@{}}
\toprule
Family & Representative result & Gate \\
\midrule
CT teacher u.b. & Mid $+0.045$ [$+0.019,+0.069$]; 3-slice $+0.051$ [$+0.025,+0.080$] & Pass \\
JDCNet & 3-slice soft-KL $+0.0345$ [$+0.0112,+0.0571$]; mid hard $+0.0329$ [$+0.0074,+0.0584$] & Pass (2/16) \\
Gated logit KD & Mid $-0.022$ [$-0.055,+0.011$]; DRR $-0.064$ [$-0.095,-0.034$] & Fail \\
Contrastive align. & Best cell $+0.008$ [$-0.020,+0.037$] & Fail \\
BiomedCLIP fine-tune & $+0.002$ [$-0.048,+0.050$] & Fail \\
Historical 226 ref. & Near-pass $+0.034$, CI crosses zero & Hist. \\
\bottomrule
\end{tabularx}
\end{table}

The CT teacher rows rule out the trivial explanation that CT carries no additional information; the negative logit and contrastive rows rule out the opposite over-generalization that any CT-to-X-ray objective will work. The supported claim lies between: confidence-gated auxiliary targets transfer a measurable fraction of the CT head-room in this paired cohort, and this evidence should be replicated before broader deployment claims.

\subsection{Full Contrastive-Alignment Sweep}
\label{sec:app_contrastive_510}

Only the best contrastive-alignment cell is shown in Table~\ref{tab:app_comparator_summary}. Table~\ref{tab:app_contrastive_510} reports the complete 4-cell sweep so that the search budget is fully visible. Two teacher representations (mid-slice and 3-slice stack, the two views that pass the teacher upper-bound gate) and two InfoNCE temperatures ($\tau\in\{0.07,0.20\}$) are evaluated under the same 5-fold patient-level CV, seeds 42--44, ResNet-18 student, weighted sampler, and gate as the JDCNet sweep. The CLIP-style two-stage protocol is: (Stage~1) train a paired CT/X-ray encoder pair plus projection heads with symmetric InfoNCE on patient-paired batches for 100 epochs; (Stage~2) discard the CT branch, replace the X-ray head with a linear classifier, and fine-tune for 50 epochs with weighted cross-entropy on the same labelled paired manifest. No cell clears the gate; the best cell (3-slice stack, $\tau{=}0.20$) yields $\Delta\mathrm{BA}=+0.008$ with $7/15$ positive cells. Mid-slice cells are negative on the point estimate. The feature-space contrastive channel therefore fails to recover the teacher upper-bound signal independently of both teacher view and temperature, strengthening the conclusion that the cross-modal bottleneck is not specific to the logit channel.

\begin{table}[htbp]
\caption{Cross-modal contrastive alignment (CLIP-style InfoNCE pretrain + supervised fine-tune) on the 510-patient BIMCV paired cohort. Each row is $n=15$ paired fold/seed cells. $\Delta\mathrm{BA}$ is the paired difference against the supervised X-ray baseline.}
\label{tab:app_contrastive_510}
\centering
\scriptsize
\setlength{\tabcolsep}{3pt}
\renewcommand{\arraystretch}{0.9}
\begin{tabularx}{\columnwidth}{@{}Xcccc@{}}
\toprule
Teacher & $\tau$ & BA mean [95\% CI] & $\Delta\mathrm{BA}$ [95\% CI] & Gate \\
\midrule
3-slice stack & 0.20 & 0.633 [0.610, 0.656] & $+0.008$ [$-0.020,+0.037$] & Fail \\
3-slice stack & 0.07 & 0.627 [0.594, 0.657] & $+0.003$ [$-0.023,+0.030$] & Fail \\
Mid-slice     & 0.20 & 0.620 [0.594, 0.643] & $-0.005$ [$-0.031,+0.020$] & Fail \\
Mid-slice     & 0.07 & 0.616 [0.590, 0.642] & $-0.008$ [$-0.038,+0.027$] & Fail \\
\bottomrule
\end{tabularx}
\end{table}

\subsection{Cross-Source Non-COVID Control}
\label{sec:app_noncovid_control}

To audit external validity outside the paired BIMCV cohort, we evaluate the cross-modal pipelines on a combined cross-source manifest: BIMCV COVID-positive CXR images (label~1) paired with up to 50 NORMAL CXR images from the public \emph{chest-xray-pneumonia} dataset (label~0, independent acquisition source). Each method is trained as in the main BIMCV protocol and then evaluated, without any cross-source fine-tuning, on 8 patient-level resamples of this mixed manifest. Table~\ref{tab:app_noncovid_control} shows that every method achieves sensitivity 1.00 on the COVID-positive class while specificity collapses toward zero on the independent NORMAL class. The ROC-AUC equals specificity in this regime because probability outputs become near-binary on out-of-distribution negatives. This is not a JDCNet-specific failure: the supervised X-ray baseline and every transfer comparator behave the same way, confirming that distribution shift between BIMCV and an unrelated normal-CXR source erases the discrimination signal. The result reinforces the main-text limitation that the present claim is a within-cohort transfer-channel finding and that external paired-cohort replication is required before any deployment interpretation.

\begin{table}[htbp]
\caption{Cross-source non-COVID control. Mean $\pm$ std over 8 patient-level resamples. ROC-AUC equals specificity because probability outputs become near-binary under distribution shift.}
\label{tab:app_noncovid_control}
\centering
\scriptsize
\setlength{\tabcolsep}{3pt}
\renewcommand{\arraystretch}{0.9}
\begin{tabularx}{\columnwidth}{@{}Xccc@{}}
\toprule
Method & Sensitivity & Specificity & ROC-AUC \\
\midrule
Supervised X-ray             & $1.00{\pm}.00$ & $0.32{\pm}.34$ & $0.32{\pm}.34$ \\
Plain cross-modal logit KD   & $1.00{\pm}.00$ & $0.00{\pm}.00$ & $0.00{\pm}.00$ \\
Attention transfer           & $1.00{\pm}.00$ & $0.10{\pm}.25$ & $0.10{\pm}.25$ \\
Feature hints                & $1.00{\pm}.00$ & $0.00{\pm}.00$ & $0.00{\pm}.00$ \\
Module-augmented pilot       & $1.00{\pm}.00$ & $0.27{\pm}.38$ & $0.27{\pm}.38$ \\
\bottomrule
\end{tabularx}
\end{table}

\subsection{CT Teacher Representation Comparison}
\label{sec:app_ct_variants}

The choice of CT teacher view---mid-slice, 3-slice stack, multi-slice mean projection, or DRR---is the most consequential design decision in the JDCNet pipeline, so we report a complete representation audit on the BIMCV-only balanced 226-patient cohort that preceded the 510-patient validation. Table~\ref{tab:app_ct_variants} reports the full $4{\times}4$ matrix (four teacher views, four method rows: teacher upper bound, supervised, plain logit KD, gated logit KD with $T{=}4$, $\tau{=}0.55$) under 5-fold patient-level CV and seeds 42--44 ($n{=}15$ cells per row). Two observations frame the 510-patient transition. First, the multi-slice projection teacher is the only representation that achieves a validated teacher upper bound at this scale ($\Delta\mathrm{BA}{=}{+}0.045$, CI $[{+}0.008,{+}0.081]$), showing that CT representation quality directly affects how much teacher signal is available. Second, no gated KD cell passes the gate for any representation: gated KD deltas range from $-0.045$ (3-slice) to $-0.005$ (DRR). The cross-modal bottleneck is therefore independent of teacher representation at this cohort scale---even the representation that satisfies the upper-bound gate does not transfer through soft logits. At 510 patients (Tier~3), this picture flips for the teacher upper bound (mid and 3-slice clear the upper-bound gate while multi-slice projection just misses), but the gated-KD failure persists across all four teachers, motivating the JDCNet confidence-gated auxiliary target.

\begin{table}[htbp]
\caption{CT teacher representation comparison on the BIMCV-only balanced 226-patient 5-fold CV ($n{=}15$ cells per row). $\Delta\mathrm{BA}$ is the paired difference against the supervised baseline trained under the same representation-specific split.}
\label{tab:app_ct_variants}
\centering
\scriptsize
\setlength{\tabcolsep}{2.5pt}
\renewcommand{\arraystretch}{0.88}
\begin{tabularx}{\columnwidth}{@{}p{0.22\columnwidth}lXc@{}}
\toprule
Teacher & Method & $\Delta\mathrm{BA}$ [95\% CI] & Gate \\
\midrule
Mid-slice            & Teacher       & $+0.012$ [$-0.024,+0.046$] & --- \\
                     & Plain KD      & $-0.022$ [$-0.062,+0.021$] & Fail \\
                     & Gated KD      & $-0.014$ [$-0.053,+0.023$] & Fail \\
3-slice stack        & Teacher       & $+0.019$ [$-0.013,+0.058$] & --- \\
                     & Plain KD      & $-0.030$ [$-0.083,+0.016$] & Fail \\
                     & Gated KD      & $-0.045$ [$-0.092,+0.000$] & Fail \\
Multi-slice proj.    & Teacher       & $\mathbf{+0.045}$ [$\mathbf{+0.008},\mathbf{+0.081}$] & \textbf{Pass} \\
                     & Plain KD      & $-0.031$ [$-0.082,+0.019$] & Fail \\
                     & Gated KD      & $-0.015$ [$-0.058,+0.027$] & Fail \\
DRR                  & Teacher       & $+0.023$ [$-0.023,+0.066$] & --- \\
                     & Plain KD      & $-0.043$ [$-0.095,+0.014$] & Fail \\
                     & Gated KD      & $-0.005$ [$-0.048,+0.039$] & Fail \\
\bottomrule
\end{tabularx}
\end{table}

\subsection{Gated Logit-KD Temperature-Threshold Scan}
\label{sec:app_calibration_scan}

We also ran a $3{\times}3$ gated-logit KD calibration scan on the 226-patient cohort ($T\in\{2,4,8\}$, $\tau\in\{0.50,0.55,0.60\}$; 8 new cells plus the primary centre cell; 120 new fold/seed runs). The closest new cell, $T{=}4$ and $\tau{=}0.50$, reached $\Delta\mathrm{BA}{=}{+}0.034$ but its CI crossed zero ($[-0.004,{+}0.073]$), while the other cells were weaker ($+0.014$ to $+0.023$) and gate activity stayed non-degenerate ($0.81{-}0.89$). Thus tuning produced only a small-cohort near-pass, not a validated transfer channel; at 510 patients the corresponding gated-logit pattern became negative. Mechanistically, the failed logit-KD, DRR, and contrastive rows show that CT confidence, geometric similarity, and embedding alignment are insufficient by themselves; only selective privileged targets transfer here, and broader generality needs multi-cohort validation.

\end{document}
